# Supplementary material for: Impacts of Antarctic fast dynamics on sea-level projections and coastal flood defense
Source: arXiv:1612.07175 ancillary file (2017-06-19)
Supplement: Supplementary file 1 [file Online_Resource_1.pdf]

**Online Resource 1, accompanying "Impacts of Antarctic Fast Dynamics on Sea-Level Projections and Coastal Flood Defense"**

Submission to *Climatic Change*

Tony E. Wong, Alexander Bakker, and Klaus Keller

Corresponding author: Tony E. Wong, 2217 EESB Pennsylvania State University, University Park, Pennsylvania, 16802, USA; twong@psu.edu

**Supplementary Figures**

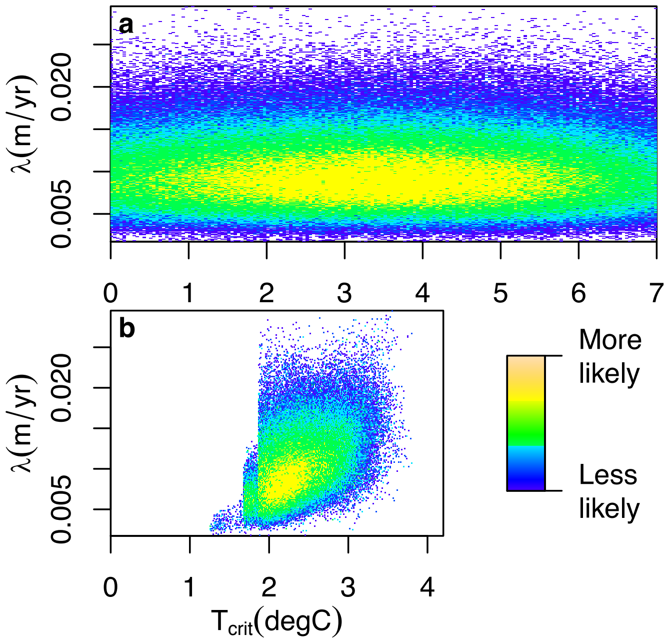


**Supplementary Figure 1 |** Pairwise prior (before the paleoclimatic calibration, panel a) and posterior (after the paleoclimatic calibration, panel b) distributions for the AIS fast dynamics parameters, assuming gamma priors.

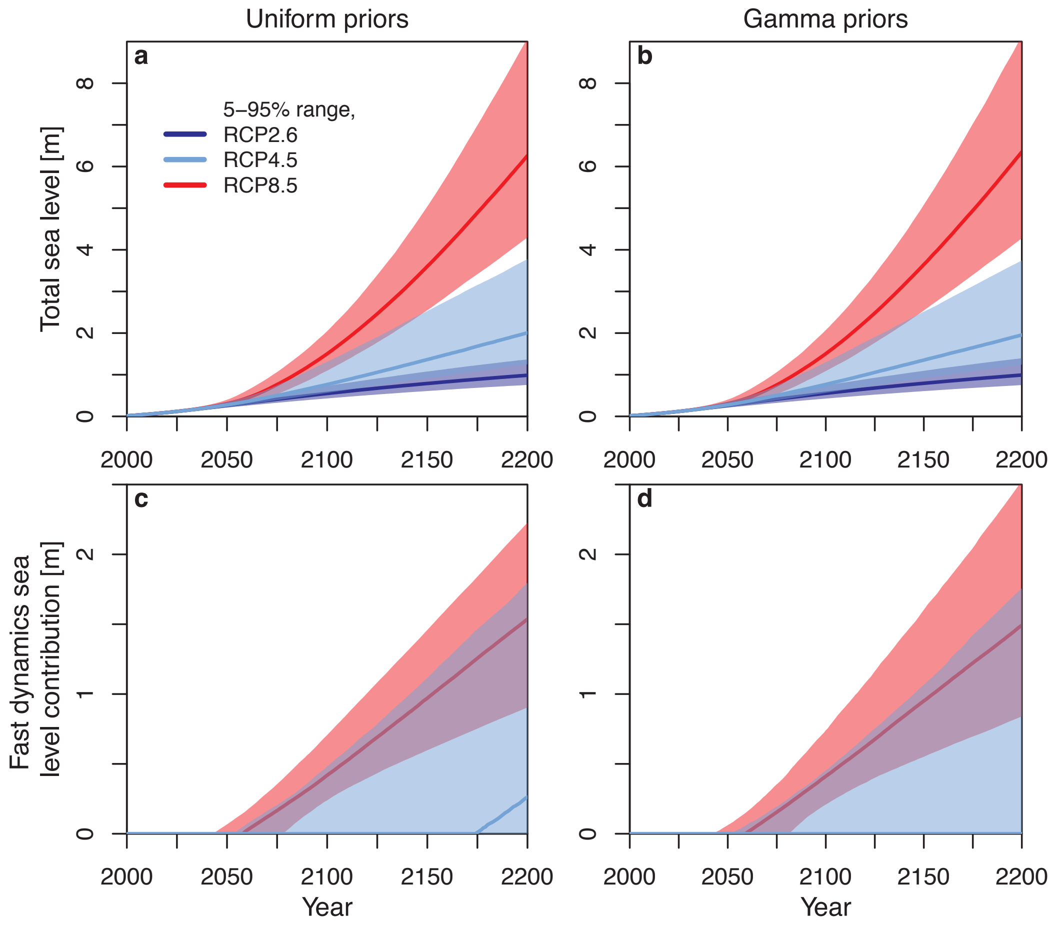


**Supplementary Figure 2** | Projections to 2200 of (top row) total sea level and (bottom row) the Antarctic fast dynamics contribution to sea-level rise, relative to the global mean 1986-2005 sea level, under RCP2.6 (blue), RCP4.5 (light blue), and RCP8.5 (red) radiative forcing scenarios. Left column: uniform priors assumed for the fast dynamics parameters; right column: gamma priors assumed.

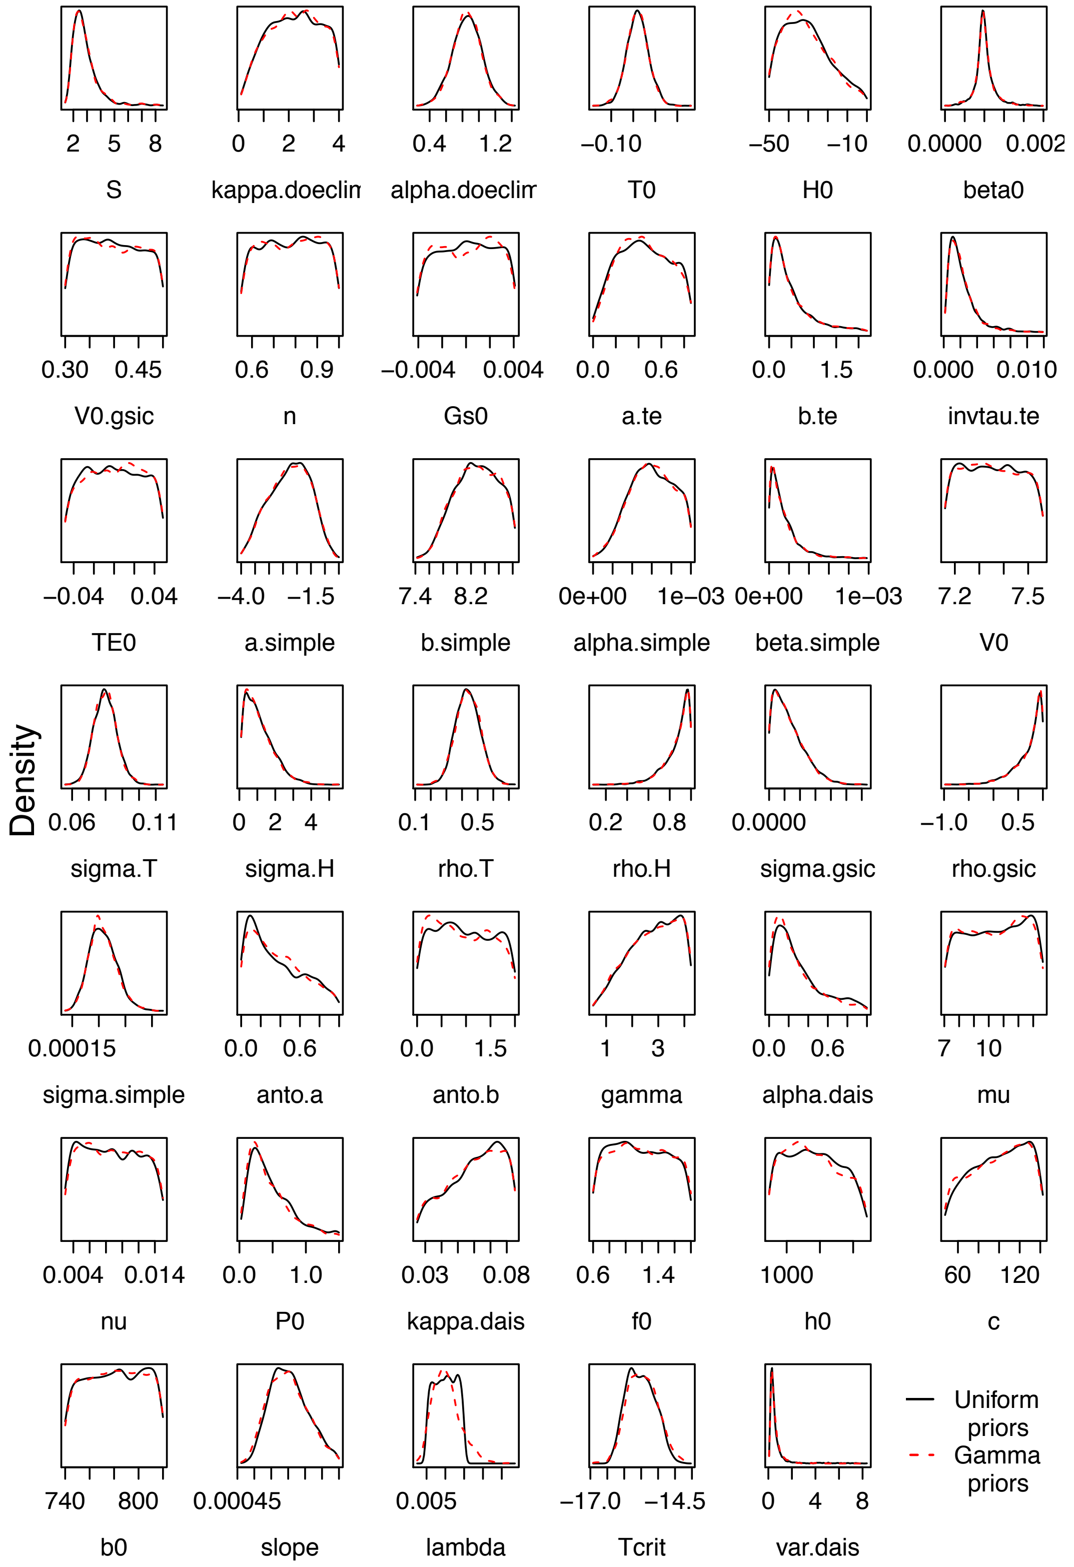


**Supplementary Figure 3 |** Calibrated parameter distributions for uniform (solid black lines) and gamma (dashed red lines) priors assumed for the fast dynamics parameters.

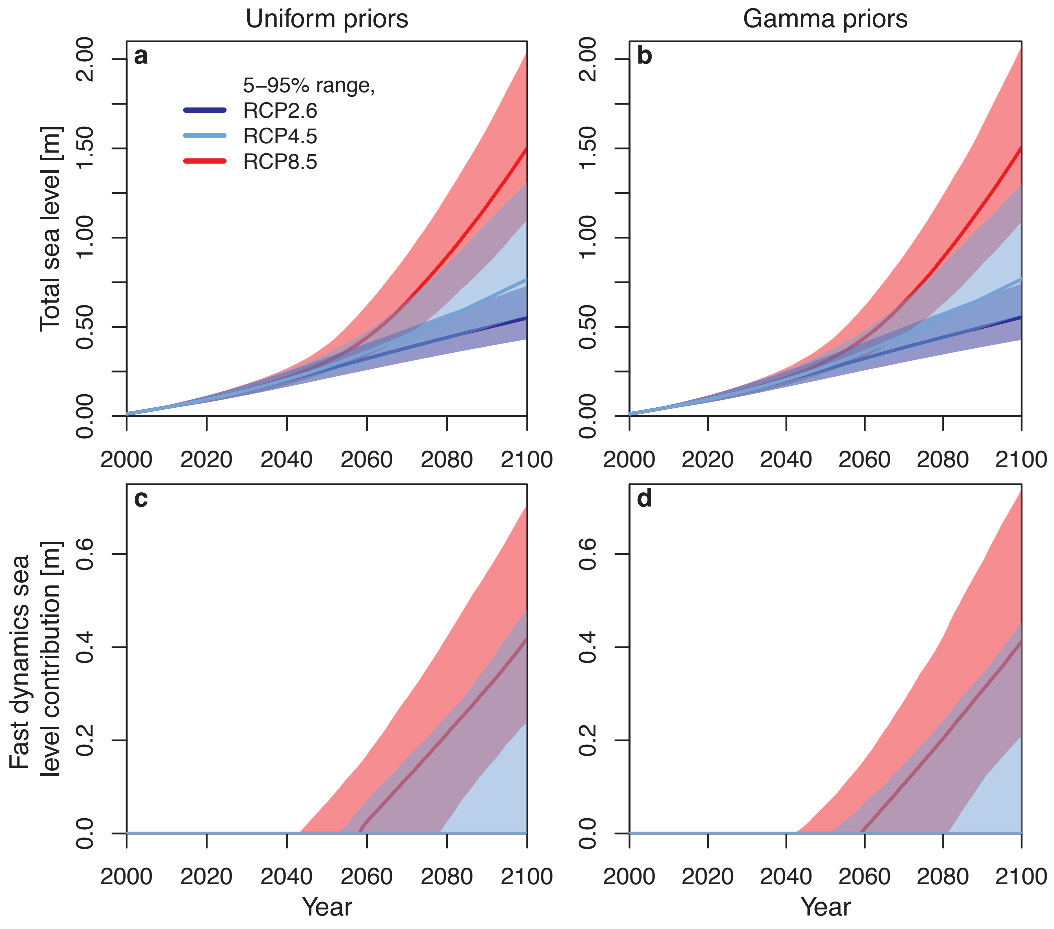


**Supplementary Figure 4 |** Projections of (top row) total sea level and (bottom row) the Antarctic fast dynamics contribution to sea-level rise, relative to the global mean 1986-2005 sea level, under RCP2.6 (blue), RCP4.5 (light blue), and RCP8.5 (red) radiative forcing scenarios. Left column: uniform priors assumed for the fast dynamics parameters; right column: gamma priors assumed.
