# Supplementary material for: Impacts of Antarctic fast dynamics on sea-level projections and coastal flood defense
Source: arXiv:1612.07175 ancillary file (2017-06-19)
Supplement: Supplementary file 2 [file Online_Resource_2.pdf]

| Parameter | Model | Median | 5% quantile | 95% quantile | Lower bound | Upper bound | Units |
|---|---|---|---|---|---|---|---|
| S | DOECLIM | 2.638 | 1.834 | 4.701 | 0.1 | 10 | deg C |
| kappa.doeclim | DOECLIM | 2.267 | 0.5769 | 3.813 | 0.1 | 4 | cm^2 s^{-1} |
| alpha.doeclim | DOECLIM | 0.8562 | 0.5712 | 1.143 | 0 | 2 | - |
| T0 | DOECLIM | -0.04042 | -0.08157 | 0.000589 | -0.3 | 0.3 | deg C |
| H0 | DOECLIM | -32.82 | -47.82 | -8.948 | -50 | 0 | 10^{22} J |
| sigma.T | DOECLIM | 0.0798 | 0.06956 | 0.09095 | 0.05 | 5 | deg C |
| sigma.H | DOECLIM | 0.9232 | 0.1824 | 2.609 | 0.1 | 10 | 10^{22} J |
| rho.T | DOECLIM | 0.4375 | 0.3099 | 0.5639 | 0 | 0.999 | - |
| rho.H | DOECLIM | 0.9094 | 0.6266 | 0.9917 | 0 | 0.999 | - |
| beta0 | GSIC | 0.00098 | 0.000619 | 0.001444 | 0 | 0.041 | m yr^{-1} deg C^{-1} |
| V0.gsic | GSIC | 0.3958 | 0.3097 | 0.4908 | 0.3 | 0.5 | m SLE |
| n | GSIC | 0.7834 | 0.577 | 0.9781 | 0.55 | 1 | - |
| Gs0 | GSIC | 0.00013 | -0.003667 | 0.003702 | -0.0041 | 0.0041 | m SLE |
| sigma.gsic | GSIC | 0.000208 | 1.62E-05 | 0.000613 | 0 | 0.0015 | m SLE |
| rho.gsic | GSIC | 0.8225 | 0.1246 | 0.9899 | -0.999 | 0.999 | - |
| a.te | TE | 0.4393 | 0.1079 | 0.8078 | 0 | 0.8595 | m deg C^{-1} |
| b.te | TE | 0.3079 | 0.02999 | 1.467 | 0 | 2.193 | m SLE |
| invtau.te | TE | 0.00179 | 0.000495 | 0.005228 | 0 | 1 | yr^{-1} |
| TE0 | TE | 0.002385 | -0.04258 | 0.04344 | -0.0484 | 0.0484 | m SLE |
| c.simple | SIMPLE-GIS | -2.219 | -3.452 | -1.155 | -4 | -0.001 | m SLE deg C^{-1} |
| b.simple | SIMPLE-GIS | 8.291 | 7.784 | 8.765 | 5.888 | 8.832 | m SLE |
| alpha.simple | SIMPLE-GIS | 0.000604 | 0.000239 | 0.00095 | 0 | 0.001 | yr^{-1} deg C^{-1} |
| beta.simple | SIMPLE-GIS | 9.88E-05 | 7.18E-06 | 0.00043 | 0 | 0.001 | yr^{-1} |
| V0 | SIMPLE-GIS | 7.352 | 7.177 | 7.539 | 7.16 | 7.56 | m SLE |
| sigma.simple | SIMPLE-GIS | 0.000205 | 0.00017 | 0.000253 | 0 | 0.002 | m SLE |
| rho.simple | SIMPLE-GIS | 0.8821 | 0.8821 | 0.8821 | 0.8821 | 0.8821 | - |
| anto.a | AntOc | 0.324 | 0.02902 | 0.8689 | 0 | 1 | deg C deg C^{-1} |
| anto.b | AntOc | 0.8959 | 0.07626 | 1.883 | 0 | 2 | deg C |
| gamma | DAIS | 2.908 | 1.17 | 4.126 | 0.5 | 4.25 | - |
| alpha.dais | DAIS | 0.1925 | 0.01959 | 0.7211 | 0 | 1 | - |
| mu | DAIS | 10.49 | 7.358 | 13.32 | 7.05 | 13.65 | m^{1/2} |
| nu | DAIS | 0.008763 | 0.00359 | 0.01433 | 0.003 | 0.015 | m^{-1/2} yr^{-1/2} |
| P0 | DAIS | 0.3548 | 0.08703 | 1.077 | 0.026 | 1.5 | m yr^{-1} |
| kappa.dais | DAIS | 0.06222 | 0.03058 | 0.08301 | 0.025 | 0.085 | deg C^{-1} |
| f0 | DAIS | 1.189 | 0.6566 | 1.744 | 0.6 | 1.8 | m yr^{-1} |
| h0 | DAIS | 1364 | 799.8 | 2086 | 735.5 | 2206.5 | m |
| c | DAIS | 101.8 | 53.83 | 137.7 | 47.5 | 142.5 | m deg C^{-1} |
| b0 | DAIS | 781.1 | 744.8 | 816.5 | 740 | 820 | m |
| slope | DAIS | 0.000597 | 0.000514 | 0.000699 | 0.00045 | 0.00075 | - |
| lambda | DAIS-FD | 0.009914 | 0.005208 | 0.01728 | 0.005 | 0.015 | m yr^{-1} |
| Tcrit | DAIS-FD | -15.47 | -16.12 | -14.71 | -20 | -10 | deg C |
| var.dais | DAIS | 0.4305 | 0.1791 | 1.499 | 0 | 2 | m^2 SLE |

| Parameter | Model | Description |
|---|---|---|
| S | DOECLIM | climate sensitivity (to doubling CO2) |
| kappa.doeclim | DOECLIM | ocean vertical diffusivity |
| alpha.doeclim | DOECLIM | aerosol scaling factor |
| T0 | DOECLIM | global mean surface temperature initial condition |
| H0 | DOECLIM | ocean heat uptake initial condition |
| sigma.T | DOECLIM | AR1 innovation standard deviation |
| sigma.H | DOECLIM | AR1 innovation standard deviation |
| rho.T | DOECLIM | autocorrelation |
| rho.H | DOECLIM | autocorrelation |
| beta0 | GSIC | initial GSIC mass balance sensitivity |
| V0.gsic | GSIC | initial GSIC volume |
| n | GSIC | exponent for area-volume scaling |
| Gs0 | GSIC | sea-level rise from GSIC in the first model year |
| sigma.gsic | GSIC | AR1 innovation standard deviation |
| rho.gsic | GSIC | autocorrelation |
| a.te | TE | temperature sensitivty of equilibrium thermal expansion |
| b.te | TE | equilibrium thermal expansion for temperature anomaly of 0 deg C |
| invtau.te | TE | 1/timescale (e-folding time) for thermal expansion response |
| TE0 | TE | initial thermal expansion |
| c.simple | SIMPLE-GIS | temperature sensitivity of equilibrium GIS volume |
| b.simple | SIMPLE-GIS | equilibrium GIS volume for temperature anomaly of 0 deg C |
| alpha.simple | SIMPLE-GIS | temperature sensitivity of GIS exponential decay rate |
| beta.simple | SIMPLE-GIS | GIS exponential decay rate for temperature anomaly of 0 deg C |
| V0 | SIMPLE-GIS | initial GIS volume |
| sigma.simple | SIMPLE-GIS | AR1 innovation standard deviation |
| rho.simple | SIMPLE-GIS | autocorrelation |
| anto.a | AntOc | sensitivity of Antarctic ocean temperature to surface temperature |
| anto.b | AntOc | Antarctic ocean temperature for surface temperature anomaly of 0 deg C |
| gamma | DAIS | power for the relation of ice flow speed to water depth |
| alpha.dais | DAIS | partition parameter for effect of ocean subsurface temperature on ice flux |
| mu | DAIS | profile parameter for parabolic Antarctic ice sheet surface (related to ice stress) |
| nu | DAIS | proportionality constant relating runoff decrease with height to precipitation |
| P0 | DAIS | Antarctic annual precipitation for Antarctic surface temperature of 0 deg C |
| kappa.dais | DAIS | coefficient for exponential dependency of precipitation on Antarctic temperature |
| f0 | DAIS | proportionality constant for ice flow at grounding line |
| h0 | DAIS | height of runoff line at Antarctic surface temperature of 0 deg C |
| c | DAIS | sensitivity of height of runoff line |
| b0 | DAIS | undisturbed bed height at the Antarctic continent center |
| slope | DAIS | slope of ice sheet bed before loading |
| lambda | DAIS-FD | Antarctic fast dynamics disintegration rate (only when temperature > Tcrit) |
| Tcrit | DAIS-FD | temperature triggering Antarctic fast dynamics disintegration |
| var.dais | DAIS | paleoclimate calibration structural uncertainty |
